# Supplementary material for: Competing nucleation pathways in nanocrystal formation
Source: arXiv:2407.05931 source file (2024-07-08)
Supplement: Supplementary file 1 [file SI.pdf]

# Competing nucleation pathways in nanocrystal formation

---

## Supplementary Information

Carlos R. Salazar,<sup>1,2</sup> Akshay Krishna Ammothum Kandy,<sup>2</sup> Jean Furstoss,<sup>1</sup> Quentin Gromoff,<sup>2</sup> Jacek Goniakowski,<sup>3</sup> and Julien Lam<sup>1,2,\*</sup>

<sup>1</sup>*Univ. Lille, CNRS, INRA, ENSCL, UMR 8207, UMET,  
Unité Matériaux et Transformations, F 59000 Lille, France*

<sup>2</sup>*Centre d'élaboration des Matériaux et d'Etudes Structurales,  
CNRS (UPR 8011), 29 rue Jeanne Marvig, 31055 Toulouse Cedex 4, France*

<sup>3</sup>*CNRS, Sorbonne Université, Institut des NanoSciences de Paris,  
UMR 7588, 4 Place Jussieu, F-75005 Paris, France*

---

\* julien.lam@cnrs.fr

### A. RELAXATION PARAMETERS

| System size | Duration relaxation steps | Duration Langevin thermostat | Relaxation temperature                | Duration Nose-Hoover thermostat    |
|-------------|---------------------------|------------------------------|---------------------------------------|------------------------------------|
| 2000 atoms  | 8 ps                      | 2 ps                         | 1350 K and 1250 K for smaller systems | 32 ps                              |
| 1500 atoms  | 7 ps                      | 2 ps                         | 1300 K                                | 34 ps                              |
| 1000 atoms  | 6 ps                      | 1 ps                         | 1200 K                                | 37 ps                              |
| 500 atoms   | 5 ps                      | 1 ps                         | 1000 K                                | 39 ps and 89 ps for larger systems |

TABLE I. Parameters used in the relaxation step for the different system sizes.

## B. ADDITIONAL BRUTE-FORCE SIMULATIONS

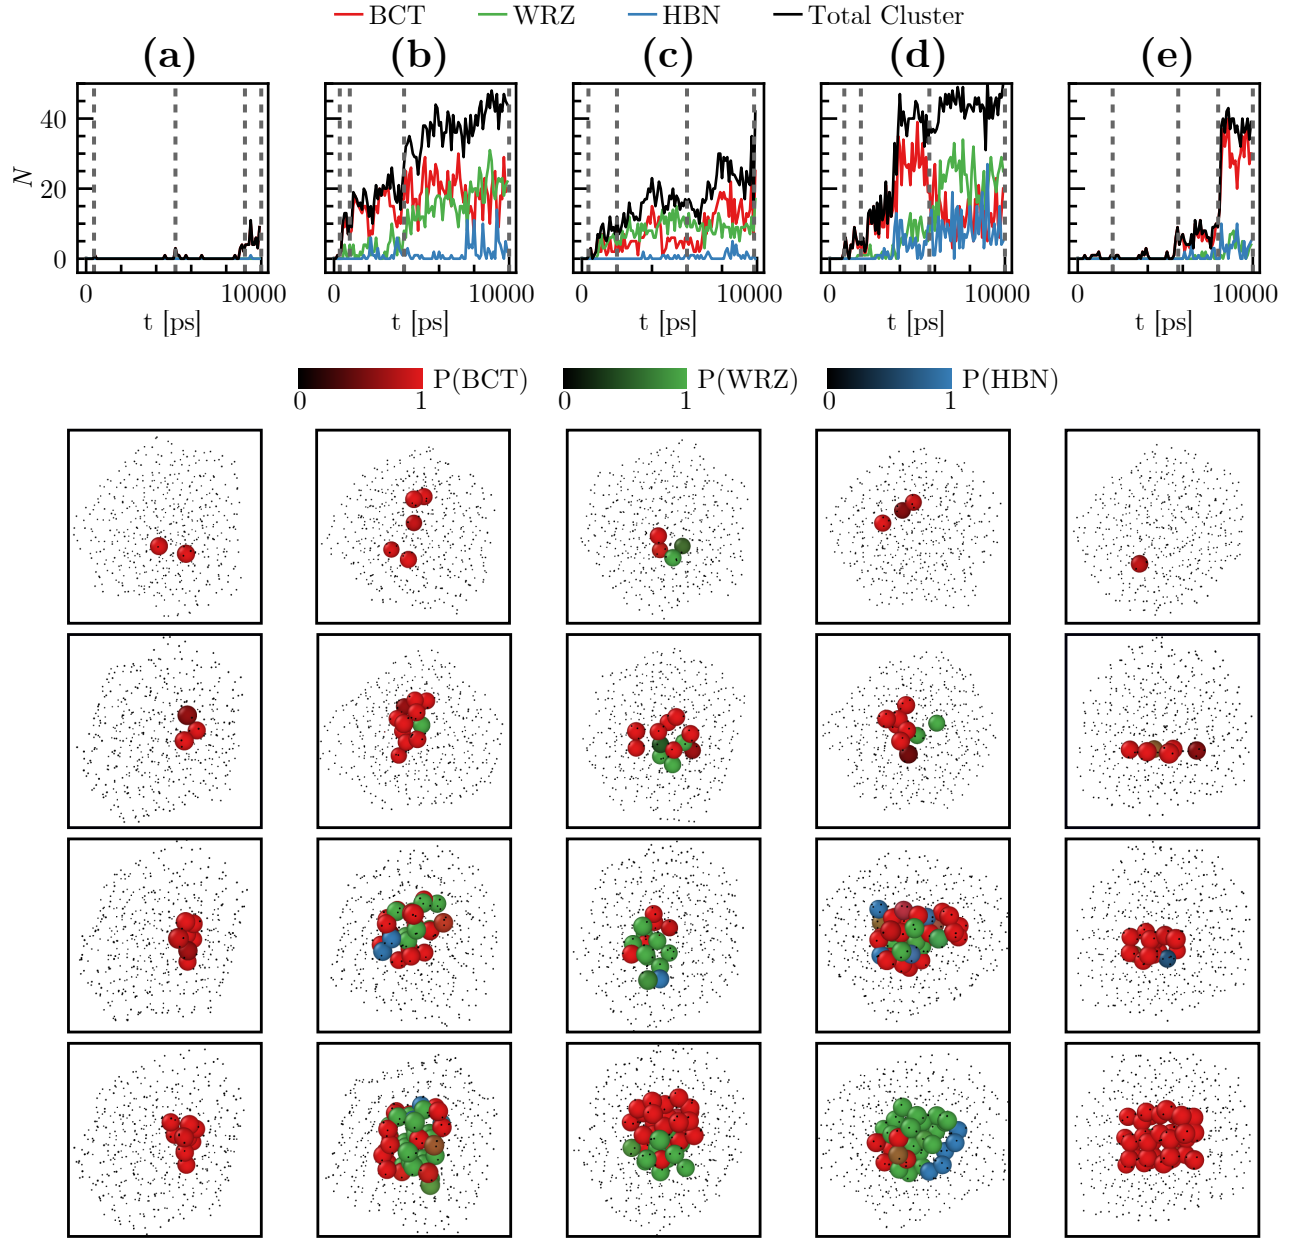

FIG. 1. Brute force nucleation simulations of ZnO nanoparticles made of 500 atoms. Five simulations are shown using different random seeds for the initial velocities in graphs (a) - (e) where the simulation time is shown on the x-axis and the number of atoms is shown on the y-axis. Snapshots of the clusters are shown below each graph corresponding to times indicated by the vertical dashed lines. Atoms are colored according to their probabilities to be in BCT structure (red), WRZ structure (green), and HBN structure (blue).

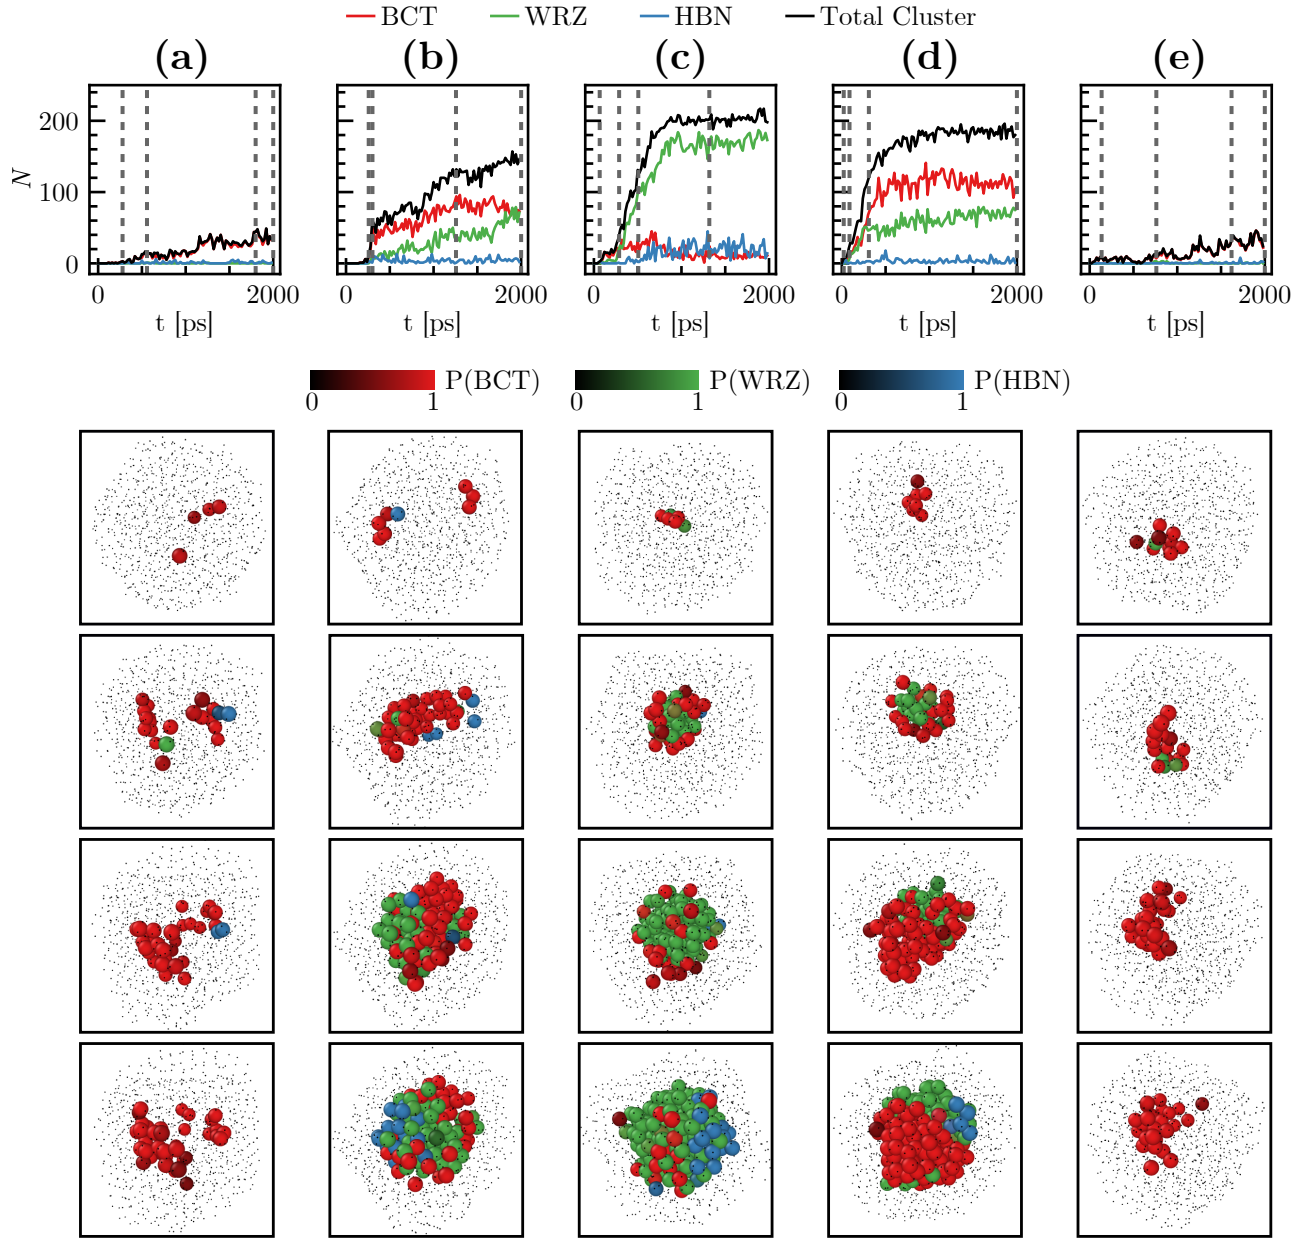

FIG. 2. Brute force nucleation simulations of ZnO nanoparticles made of 1000 atoms. Five simulations are shown using different random seeds for the initial velocities in graphs (a) - (e) where the simulation time is shown on the x-axis and the number of atoms is shown on the y-axis. Snapshots of the clusters are shown below each graph corresponding to times indicated by the vertical dashed lines. Atoms are colored according to their probabilities to be in BCT structure (red), WRZ structure (green), and HBN structure (blue).

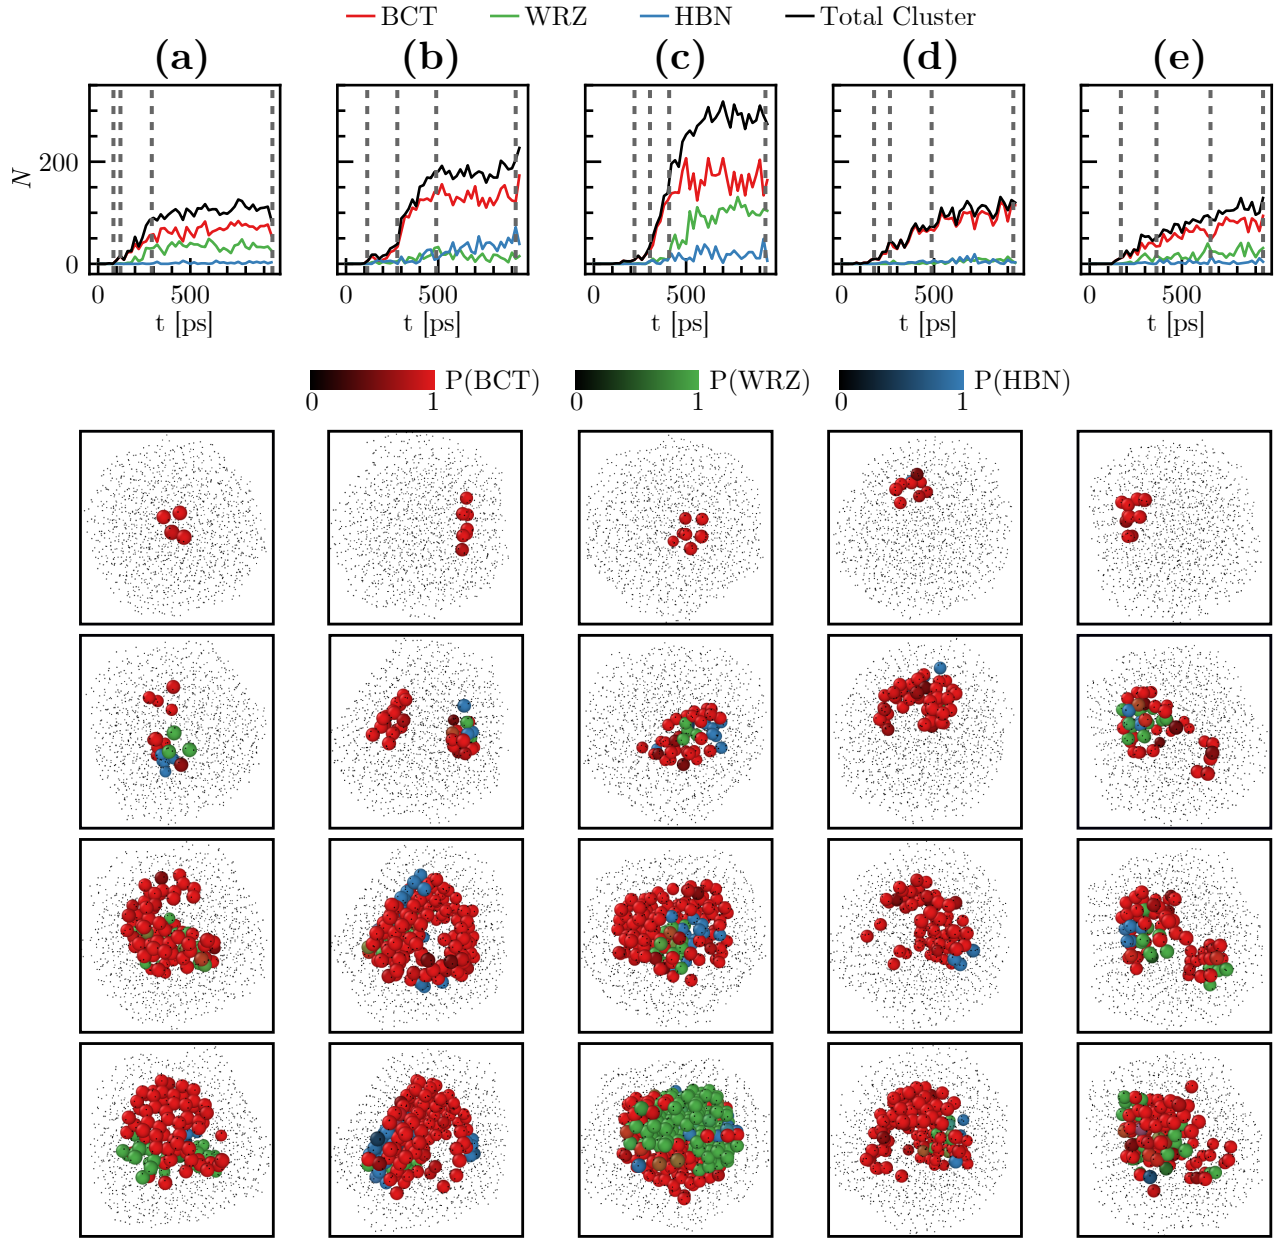

FIG. 3. Brute force nucleation simulations of ZnO nanoparticles made of 1500 atoms. Five simulations are shown using different random seeds for the initial velocities in graphs (a) - (e) where the simulation time is shown on the x-axis and the number of atoms is shown on the y-axis. Snapshots of the clusters are shown below each graph corresponding to times indicated by the vertical dashed lines. Atoms are colored according to their probabilities to be in BCT structure (red), WRZ structure (green), and HBN structure (blue).

### C. SEEDING SIMULATIONS FOR DIFFERENT DROPLET SIZES

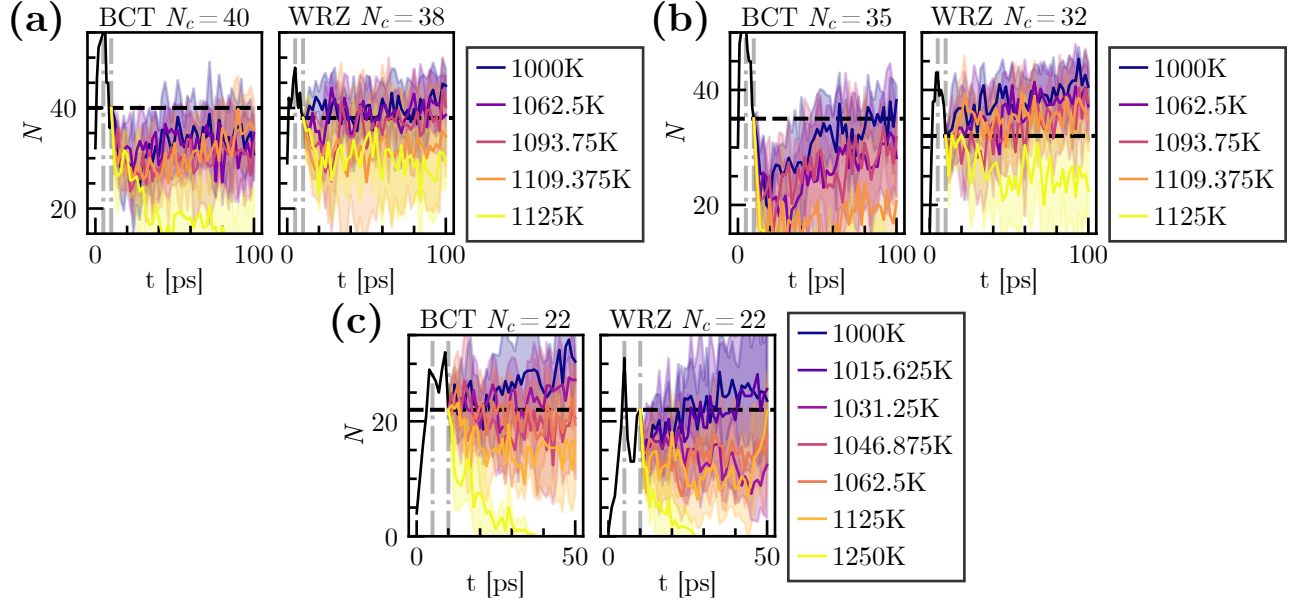

FIG. 4. Growth/Melt simulations of 500 atoms for BCT and WRZ clusters of different sizes are shown in subfigures (a) - (c). The relaxation steps are shown in each graph with a black line, after which the growth/melt simulations are shown for different temperatures. In each subfigure, two clusters of similar critical cluster size  $N_c$  but different crystal structures are compared.

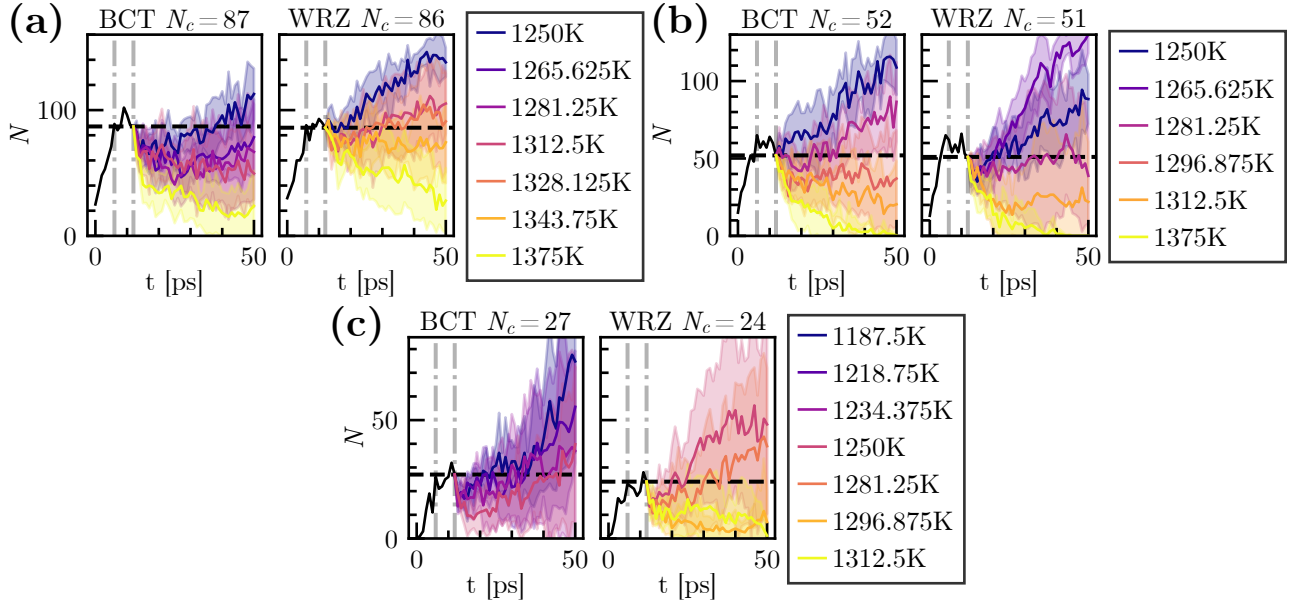

FIG. 5. Growth/Melt simulations of 1000 atoms for BCT and WRZ clusters of different sizes are shown in subfigures (a) - (c). The relaxation steps are shown in each graph with a black line, after which the growth/melt simulations are shown for different temperatures. In each subfigure, two clusters of similar critical cluster size  $N_c$  but different crystal structures are compared.

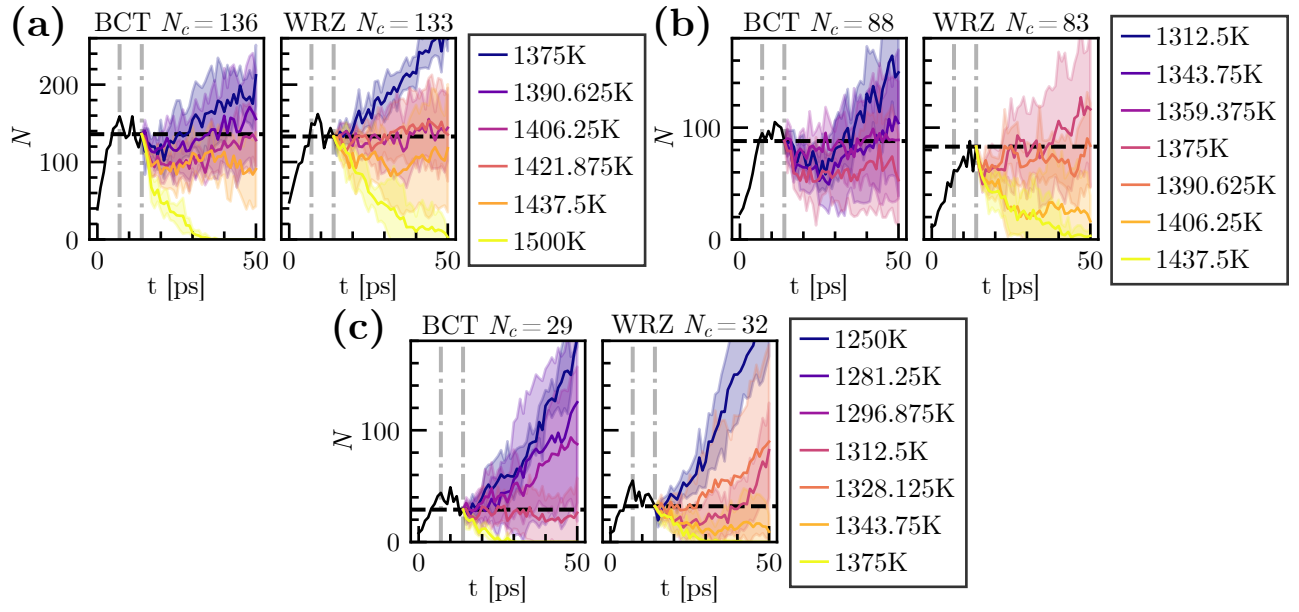

FIG. 6. Growth/Melt simulations of 1500 atoms for BCT and WRZ clusters of different sizes are shown in subfigures (a) - (c). The relaxation steps are shown in each graph with a black line, after which the growth/melt simulations are shown for different temperatures. In each subfigure, two clusters of similar critical cluster size  $N_c$  but different crystal structures are compared.
